# Supplementary material for: Phenotypic robustness can increase phenotypic variability after non-genetic perturbations in gene regulatory circuits
Source: arXiv:1010.0370 ancillary file (2010-10-02)
Supplement: Supplementary file 1 [file Sup.pdf]

# Supporting information for: Phenotypic robustness can increase phenotypic variability after non-genetic perturbations in gene regulatory circuits

Carlos Espinosa-Soto    Olivier C. Martin    Andreas Wagner

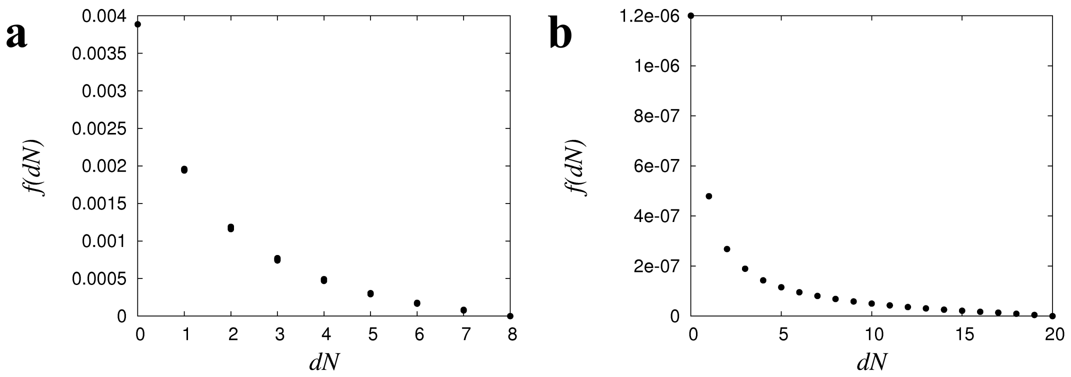


**Fig. S1.** The fraction of genotypes ($f(dN)$) that produce a phenotype decreases with $dN$. $dN$ represents the number of gene activity differences between a predetermined initial condition, $s_0$, and the phenotype $s_\infty$. To generate the data in this figure we constructed random genotypes with a specific number of genes $N$ and with a specific number of regulatory interactions $m$. (a) $N = 8; m = 23$. Sampling included $2 \times 10^7$ genotypes. Spearman's $\rho = -0.978$; $p < 2.2 \times 10^{-16}$. Each point in the plot represents a specific phenotype. (b) $N = 20; m = 85$. Sampling included $10^8$ genotypes. Spearman's $\rho = -1$; $p < 1.98 \times 10^{-6}$. Each point in the plot stands for the frequency of obtaining phenotypes with a given $d$, divided by the number of possible phenotypes with this distance $d$. All the phenotypes with equal $d$ are equally frequent (Ciliberti, Martin & Wagner, 2007, PLoS Comput Biol, 3:e15). The number of phenotypes at a distance $d$ from the fixed initial state $s_0$ is given by the binomial coefficient $\mathbf{C}_k^N$, where $k = dN$ stands for the number of gene expression differences between $s_0$ and $s_\infty$.

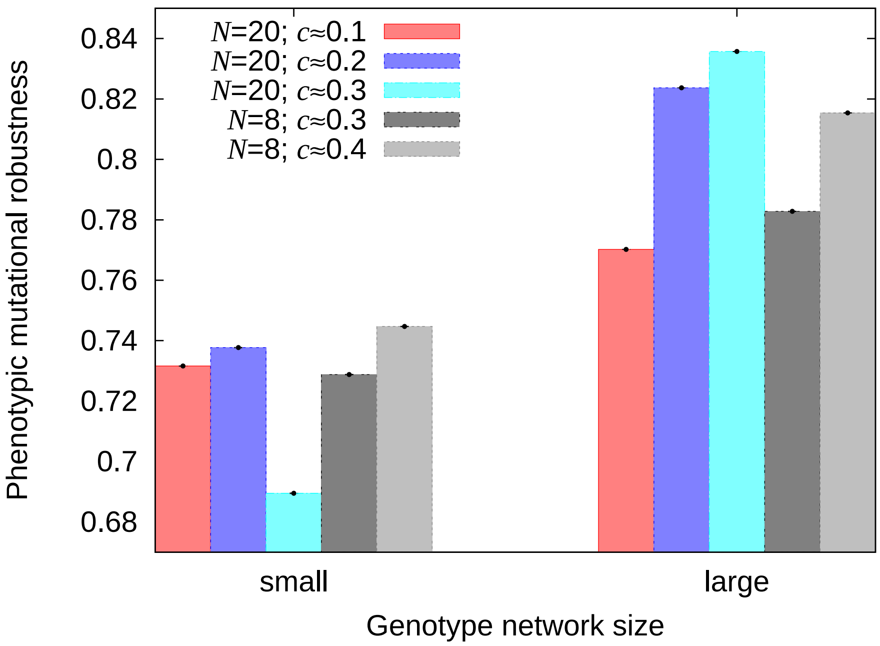


**Fig. S2.** Phenotypic mutational robustness increases with genotype network size. For the purpose of this figure, small genotype network size corresponds to $d = 0.5$. Large genotype network size corresponds to $d = 0.125$ when $N = 8$, and to $d = 0.1$ when $N = 20$. Hereafter we will refer to phenotypic mutational robustness as "phenotypic robustness". We sampled $10^6$ genotypes in each genotype network. The length of bars represents one standard error.

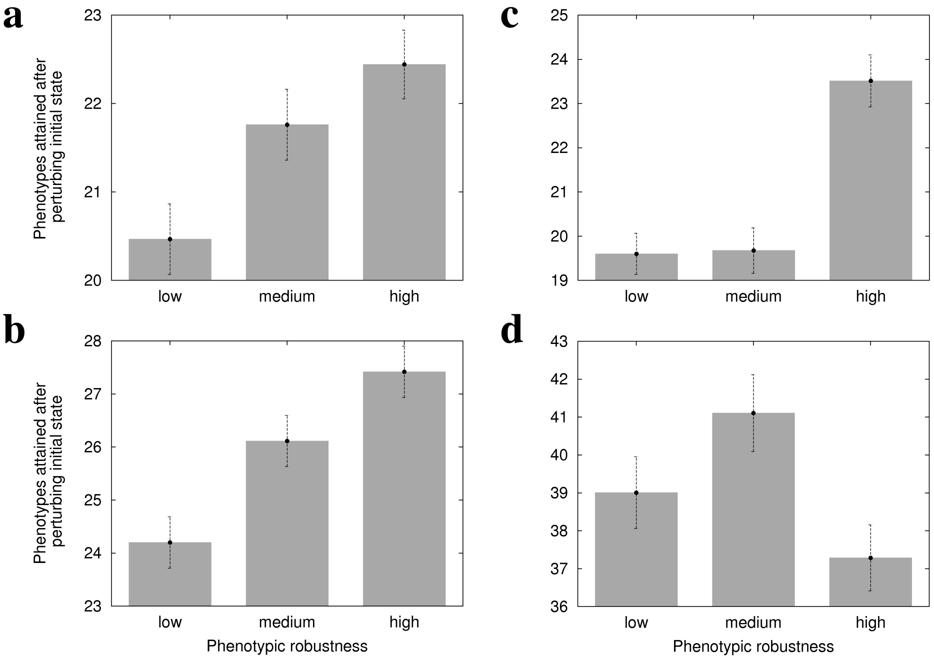


**Fig. S3.** High phenotypic robustness facilitates phenotypic variability in response to gene expression noise in $s_0$. Each plot shows mean values for 500 independent simulations at each level of phenotypic robustness. The length of bars denotes one standard error. (a) $N = 8$; $c \approx 0.4$. (b) $N = 8$; $c \approx 0.3$. (c) $N = 20$; $c \approx 0.3$. (d) $N = 20$; $c \approx 0.1$. In this and all other figures, low phenotypic robustness corresponds to $d = 0.5$, medium robustness corresponds to $d = 0.25$; high robustness corresponds to $d = 0.125$ when $N = 8$, and to $d = 0.1$ when $N = 20$.

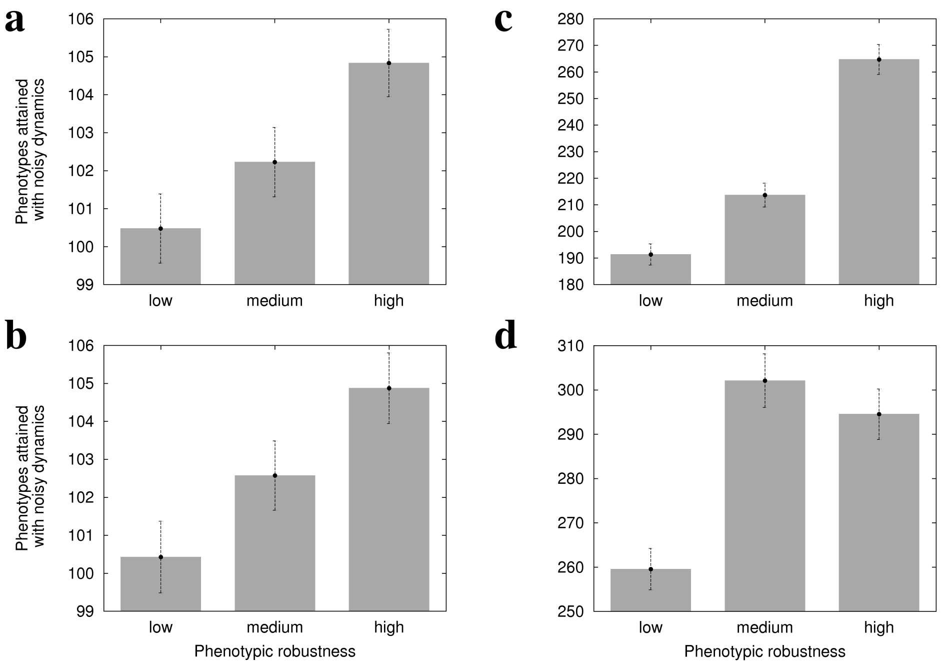


**Fig. S4.** High phenotypic robustness facilitates phenotypic variability in response to noisy gene expression dynamics. Each plot shows mean values for 500 independent simulations at each level of phenotypic robustness. The length of bars denotes one standard error. (a) $N = 8$; $c \approx 0.4$. (b) $N = 8$; $c \approx 0.3$. (c) $N = 20$; $c \approx 0.3$. (d) $N = 20$; $c \approx 0.1$.

**Table S1.** The mean and maximum genetic distance within a population increases with phenotypic robustness according to a Mann-Whitney U test.

| Genotype network $N$ | $c$ | $d$ | Mean genetic distance ±SE | P-value | Maximum genetic distance ±SE | P-value |
|---|---|---|---|---|---|---|
| 20 | 0.1 | 0.1 | 0.557±0.003 | 0.0059 | 0.874±0.003 | 9.65×10$^{-5}$ |
| | | 0.5 | 0.545±0.003 | | 0.854±0.003 | |
| | 0.2 | 0.1 | 0.434±0.003 | 3.59×10$^{-5}$ | 0.739±0.005 | 0.0056 |
| | | 0.5 | 0.415±0.003 | | 0.719±0.005 | |
| | 0.3 | 0.1 | 0.349±0.003 | 0.002 | 0.622±0.006 | 0.0056 |
| | | 0.5 | 0.334±0.003 | | 0.601±0.005 | |
| 8 | 0.3 | 0.125 | 0.697±0.002 | 4.17×10$^{-14}$ | 0.97±0.001 | 1.74×10$^{-14}$ |
| | | 0.5 | 0.675±0.002 | | 0.957±0.001 | |
| | 0.4 | 0.125 | 0.61 ±0.003 | 4.97×10$^{-7}$ | 0.901±0.002 | 5.22×10$^{-10}$ |
| | | 0.5 | 0.593±0.002 | | 0.886±0.002 | |

Mean and maximum genetic distance values are averaged across 500 populations for each combination of $N$, $c$ and $d$. Each population includes 200 gene circuits. Values of $d = 0.5$ correspond to low phenotypic robustness, and values of $d = 0.1$ or $d = 0.125$ correspond to high phenotypic robustness.

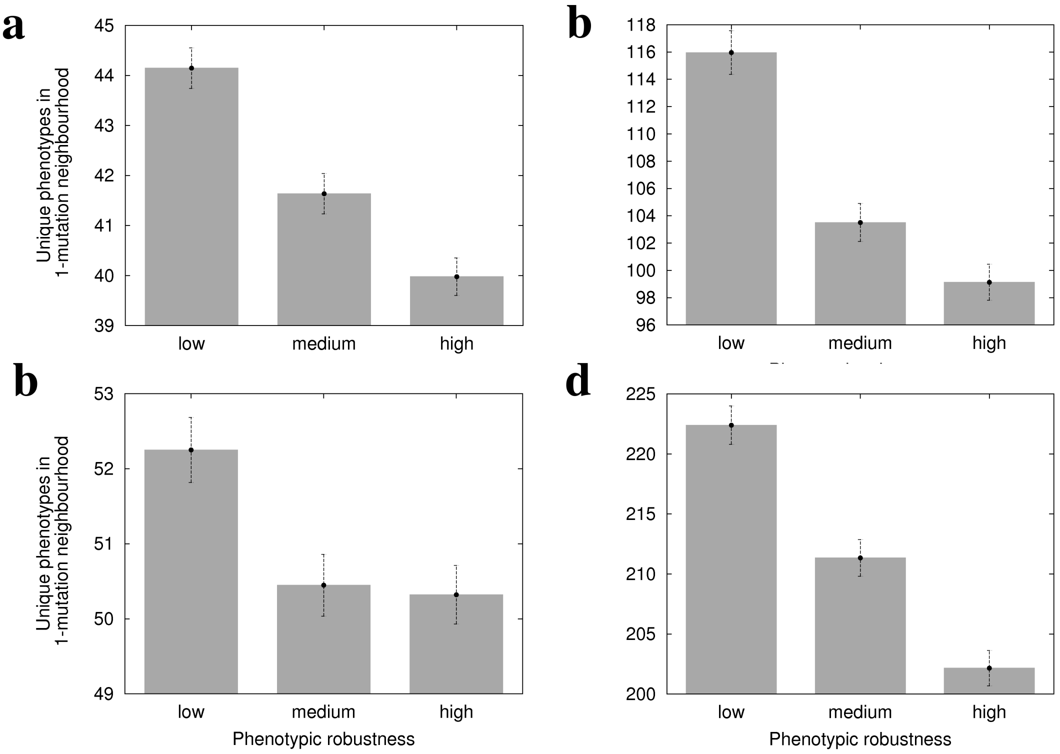


**Fig. S5.** High phenotypic robustness does not facilitate phenotypic variability in response to mutations without preceding environmental change. Each plot shows mean values for 500 independent simulations at each level of phenotypic robustness. The length of bars denotes one standard error. (a) $N = 8$; $c \approx 0.4$. (b) $N = 8$; $c \approx 0.3$. (c) $N = 20$; $c \approx 0.3$. (d) $N = 20$; $c \approx 0.1$.

**Table S2.** Mean number of new phenotypes accessible from individual genotypes in populations evolving in different genotype networks.

| Genotype network | | | Mean number of new phenotypes ± SE | | |
|---|---|---|---|---|---|
| $N$ | $c$ | $d$ | Mutation | Perturbing $s_0$ | Noisy dynamics |
| 20 | 0.1 | 0.1 | $6.5 \pm 0.04$ | $1.01 \pm 0.03$ | $6.97 \pm 0.11$ |
| | | 0.5 | $7.3 \pm 0.04$ | $1.17 \pm 0.03$ | $6.53 \pm 0.08$ |
| | 0.2 | 0.1 | $5.59 \pm 0.04$ | $0.86 \pm 0.02$ | $7.24 \pm 0.11$ |
| | | 0.5 | $6.46 \pm 0.05$ | $0.88 \pm 0.02$ | $6.66 \pm 0.08$ |
| | 0.3 | 0.1 | $4.33 \pm 0.04$ | $0.77 \pm 0.02$ | $7.34 \pm 0.12$ |
| | | 0.5 | $5.32 \pm 0.05$ | $0.91 \pm 0.01$ | $6.42 \pm 0.09$ |
| 8 | 0.3 | 0.125 | $2.17 \pm 0.02$ | $0.97 \pm 0.02$ | $4.99 \pm 0.04$ |
| | | 0.5 | $2.55 \pm 0.02$ | $1.05 \pm 0.02$ | $4.93 \pm 0.04$ |
| | 0.4 | 0.125 | $1.84 \pm 0.02$ | $0.81 \pm 0.02$ | $5.02 \pm 0.05$ |
| | | 0.5 | $2.33 \pm 0.02$ | $0.95 \pm 0.01$ | $5.07 \pm 0.05$ |

For each genotype network we evolved 500 independent populations. Each population includes 200 gene circuits. For each population evolved under stabilizing selection on an optimal gene activity phenotype $s_\infty^{opt}$ (see Methods in the main text), we counted the number of new phenotypes (due to mutation or non-genetic perturbations) that are within reach of each genotype in the population.

**Table S3.** Relative phenotypic variability of genotypes in large genotype networks. We define this number as the number of new phenotypes that noise and mutation can produce per genotype in populations on a large genotype network for each new phenotype produced by the same kind of perturbation, but for populations on a smaller genotype network. This ratio is always greater for noise than for mutations, with one exception[a]. Numbers on this table based on data in Table S2.

| Genotype network | | Relative phenotypic variability of genotypes in large genotype networks. | | |
|---|---|---|---|---|
| $N$ | $c$ | Mutation | Perturbing $s_0$ | Noisy dynamics |
| 20 | 0.1 | 0.891 | 0.859[a] | 1.068 |
| | 0.2 | 0.865 | 0.972 | 1.088 |
| | 0.3 | 0.815 | 0.846 | 1.143 |
| 8 | 0.3 | 0.85 | 0.917 | 1.011 |
| | 0.4 | 0.79 | 0.846 | 0.991 |

[a] The only exception occurs for very low interaction densities ($N = 20; c \approx 0.1$; and perturbations in $s_0$), where in earlier analyses, populations had also not shown higher variability when evolving on large genotype networks (Fig. S3d).

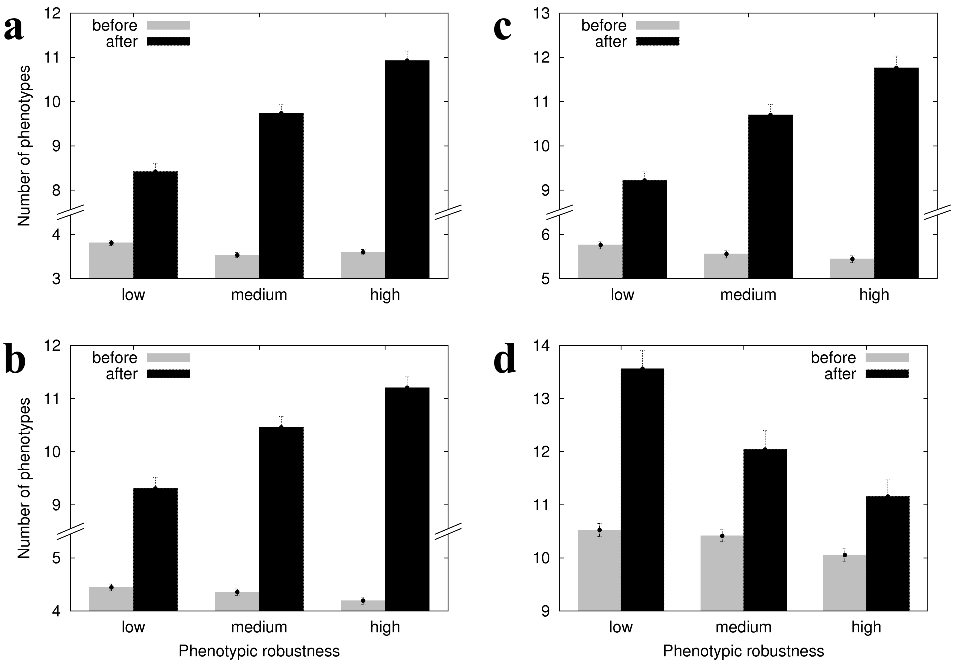


**Fig. S6.** High phenotypic robustness increases phenotypic diversity in populations of gene circuits after environmental change. The number of different phenotypes that populations display increases after shifting $s_0$. Such an increase is greater for populations with more robust phenotypes. Each plot shows mean values for 500 independent populations at each level of phenotypic robustness. The length of bars denotes one standard error. (a) $N = 8$; $c \approx 0.4$. (b) $N = 8$; $c \approx 0.3$. (c) $N = 20$; $c \approx 0.3$. (d) $N = 20$; $c \approx 0.1$.

**Table S4.** The increase in the number of different phenotypes after changing $s_0$ is larger in circuits with robust phenotypes according to a Mann-Whitney U test.

| Genotype network | | P-value[a] |
|---|---|---|
| $N$ | $c$ | |
| 20 | 0.2 | $7.8 \times 10^{-5}$ |
| | 0.3 | $1.49 \times 10^{-18}$ |
| 8 | 0.3 | $5.91 \times 10^{-14}$ |
| | 0.4 | $3.24 \times 10^{-24}$ |

[a]The comparison is performed between populations of circuits with $d = 0.1$ and $d = 0.5$ when $N = 20$, and with $d = 0.125$ and $d = 0.5$ when $N = 8$.

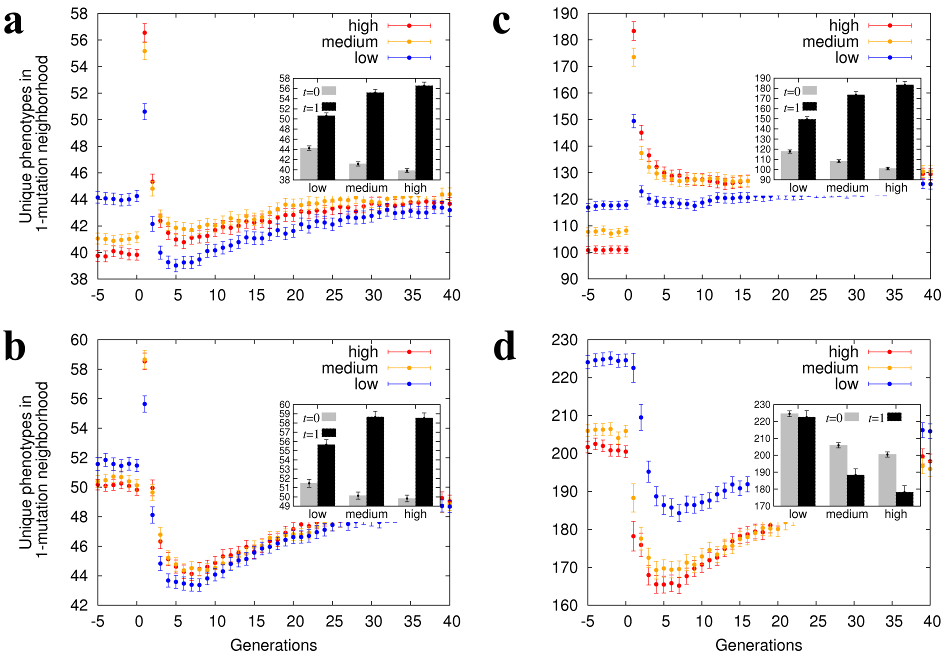


**Fig. S7.** High phenotypic robustness allows mutational access to more phenotypes after an alteration of the environment's inducing role. Each plot shows mean values of phenotypic variability for 500 independent simulations at each level of phenotypic robustness. We show in the insets the number of mutation-accessible phenotypes immediately before ($t = 0$) and immediately after ($t = 1$) replacement of $s_0$. The length of bars denotes one standard error. (a) $N = 8$; $c \approx 0.4$. (b) $N = 8$; $c \approx 0.3$. (c) $N = 20$; $c \approx 0.3$. (d) $N = 20$; $c \approx 0.1$.

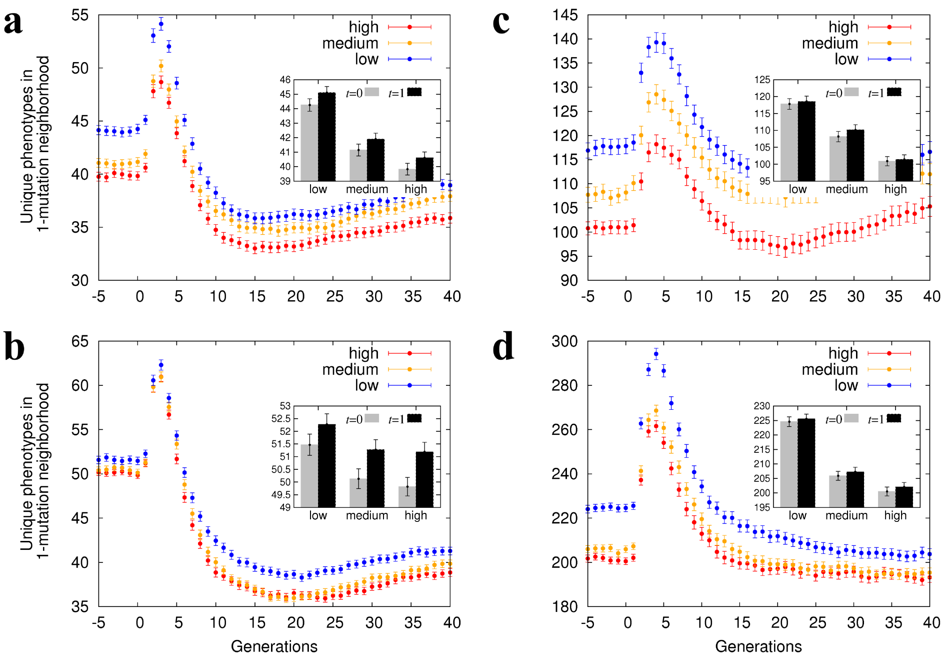


**Fig. S8.** High phenotypic robustness does not facilitate mutational access to more phenotypes after an alteration of the environment's evaluating role. Change of the evaluating role is implemented as a change in $s_{\infty}^{opt}$. Each plot shows mean values of phenotypic variability for 500 independent simulations for each level of phenotypic robustness. We show in the insets the number of mutation-accessible phenotypes immediately before ($t = 0$) and immediately after ($t = 1$) replacement of $s_{\infty}^{opt}$. The length of bars denotes one standard error. (a) $N = 8$; $c \approx 0.4$. (b) $N = 8$; $c \approx 0.3$. (c) $N = 20$; $c \approx 0.3$. (d) $N = 20$; $c \approx 0.1$.

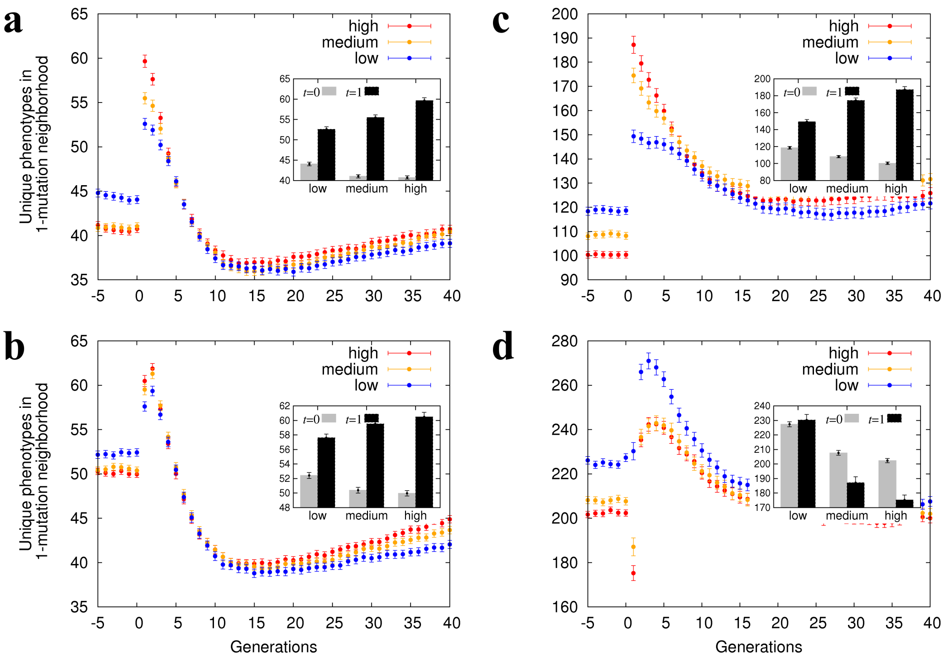


**Fig. S9.** High phenotypic robustness allows mutational access to more phenotypes after an alteration of both the inducing and evaluating role of the environment. Each plot shows mean values of phenotypic variability for 500 independent simulations for each level of phenotypic robustness. We show in the insets the number of mutation-accessible phenotypes immediately before ($t = 0$) and immediately after ($t = 1$) replacement of $s_{\infty}^{opt}$ and $s_0$. The length of bars denotes one standard error. (a) $N = 8$; $c \approx 0.4$. (b) $N = 8$; $c \approx 0.3$. (c) $N = 20$; $c \approx 0.3$. (d) $N = 20$; $c \approx 0.1$.

**Table S5.** The increase in the number of accessible new phenotypes is larger in circuits with robust phenotypes, according to a Mann-Whitney U test.

| Genotype network | | P-value[a] |
|---|---|---|
| $N$ | $c$ | |
| 20 | 0.2 | $1.78 \times 10^{-21}$ |
| | 0.3 | $5.41 \times 10^{-71}$ |
| 8 | 0.3 | $2.38 \times 10^{-16}$ |
| | 0.4 | $1.3 \times 10^{-45}$ |

[a]The comparison is performed between populations of circuits with $d = 0.1$ and $d = 0.5$ when $N = 20$, and with $d = 0.125$ and $d = 0.5$ when $N = 8$.
